# Supplementary material for: Forecaster-aided User Association and Load Balancing in Multi-band Mobile Networks
Source: arXiv:2301.09294 source file (2023-01-23)
Supplement: Supplementary file 1 [file appendix.tex]

\appendices
\section{Proof of Theorem}
\begin{proof}
Proof goes here.
\end{proof}
